# Supplementary material for: Hyper-SAGNN: a self-attention based graph neural network for hypergraphs
Source: arXiv:1911.02613 source file (2019-11-06)
Supplement: Supplementary file 1 [file Appendix.tex]

\setcounter{figure}{0}    

\setcounter{table}{0} 

\section{Appendix}
\subsection{Comparison of Our Model versus the Variants}
As mentioned above, unlike the standard GAT model, we exclude the $\alpha_{ii}$ term in the self-attention mechanism. 
To test whether this constraint would help or decrease the model's ability to learn, we implement a variant of our model (referred to as variant type I) by including this term. 
Also, as mentioned in the Method section, another potential variant of our model would be directly using the $\vec{d}^{*}_i$ to calculate the probability score $p^{*}_i$. 
We refer to this variant as variant type II. Besides these, the rest of the parameters and structure of the neural network remain the same. 
We then compared the performance of our model and two variants in terms of the AUC and AUPR value for network reconstruction task and hyperedge link prediction task on the following 4 datasets: MovieLens, wordnet, drug, and GPS. 
We also compared the performance in terms of the micro F1 score and macro F1 score on the node classification task on the MovieLens and the wordnet dataset.
For the MovieLens dataset, we used 90\% nodes as training data while for wordnet, we used 1\% of the nodes as training data.
All the test setup is the same as described in the main text. 
To avoid the effect of the randomness of the neural network training, we repeat the training process for each experiment 5 times and draw the line plot of the score versus the epoch number. 
To illustrate the differences more clearly, we start the plot at epoch 3 for the random walk based approach and epoch 12 for the encoder based approach.
The performance of the model when using the random walk based approach is shown in Fig.~\ref{fig:perform_GPS1} to Fig.~\ref{fig:perform_wordnet1}. 
The performance of the model when using the encoder based approach is shown in Figure.~\ref{fig:perform_GPS2} to Figure.~\ref{fig:perform_wordnet2}.

\begin{figure}[htbp!]
    \centering
    \includegraphics[width = 0.75\textwidth]{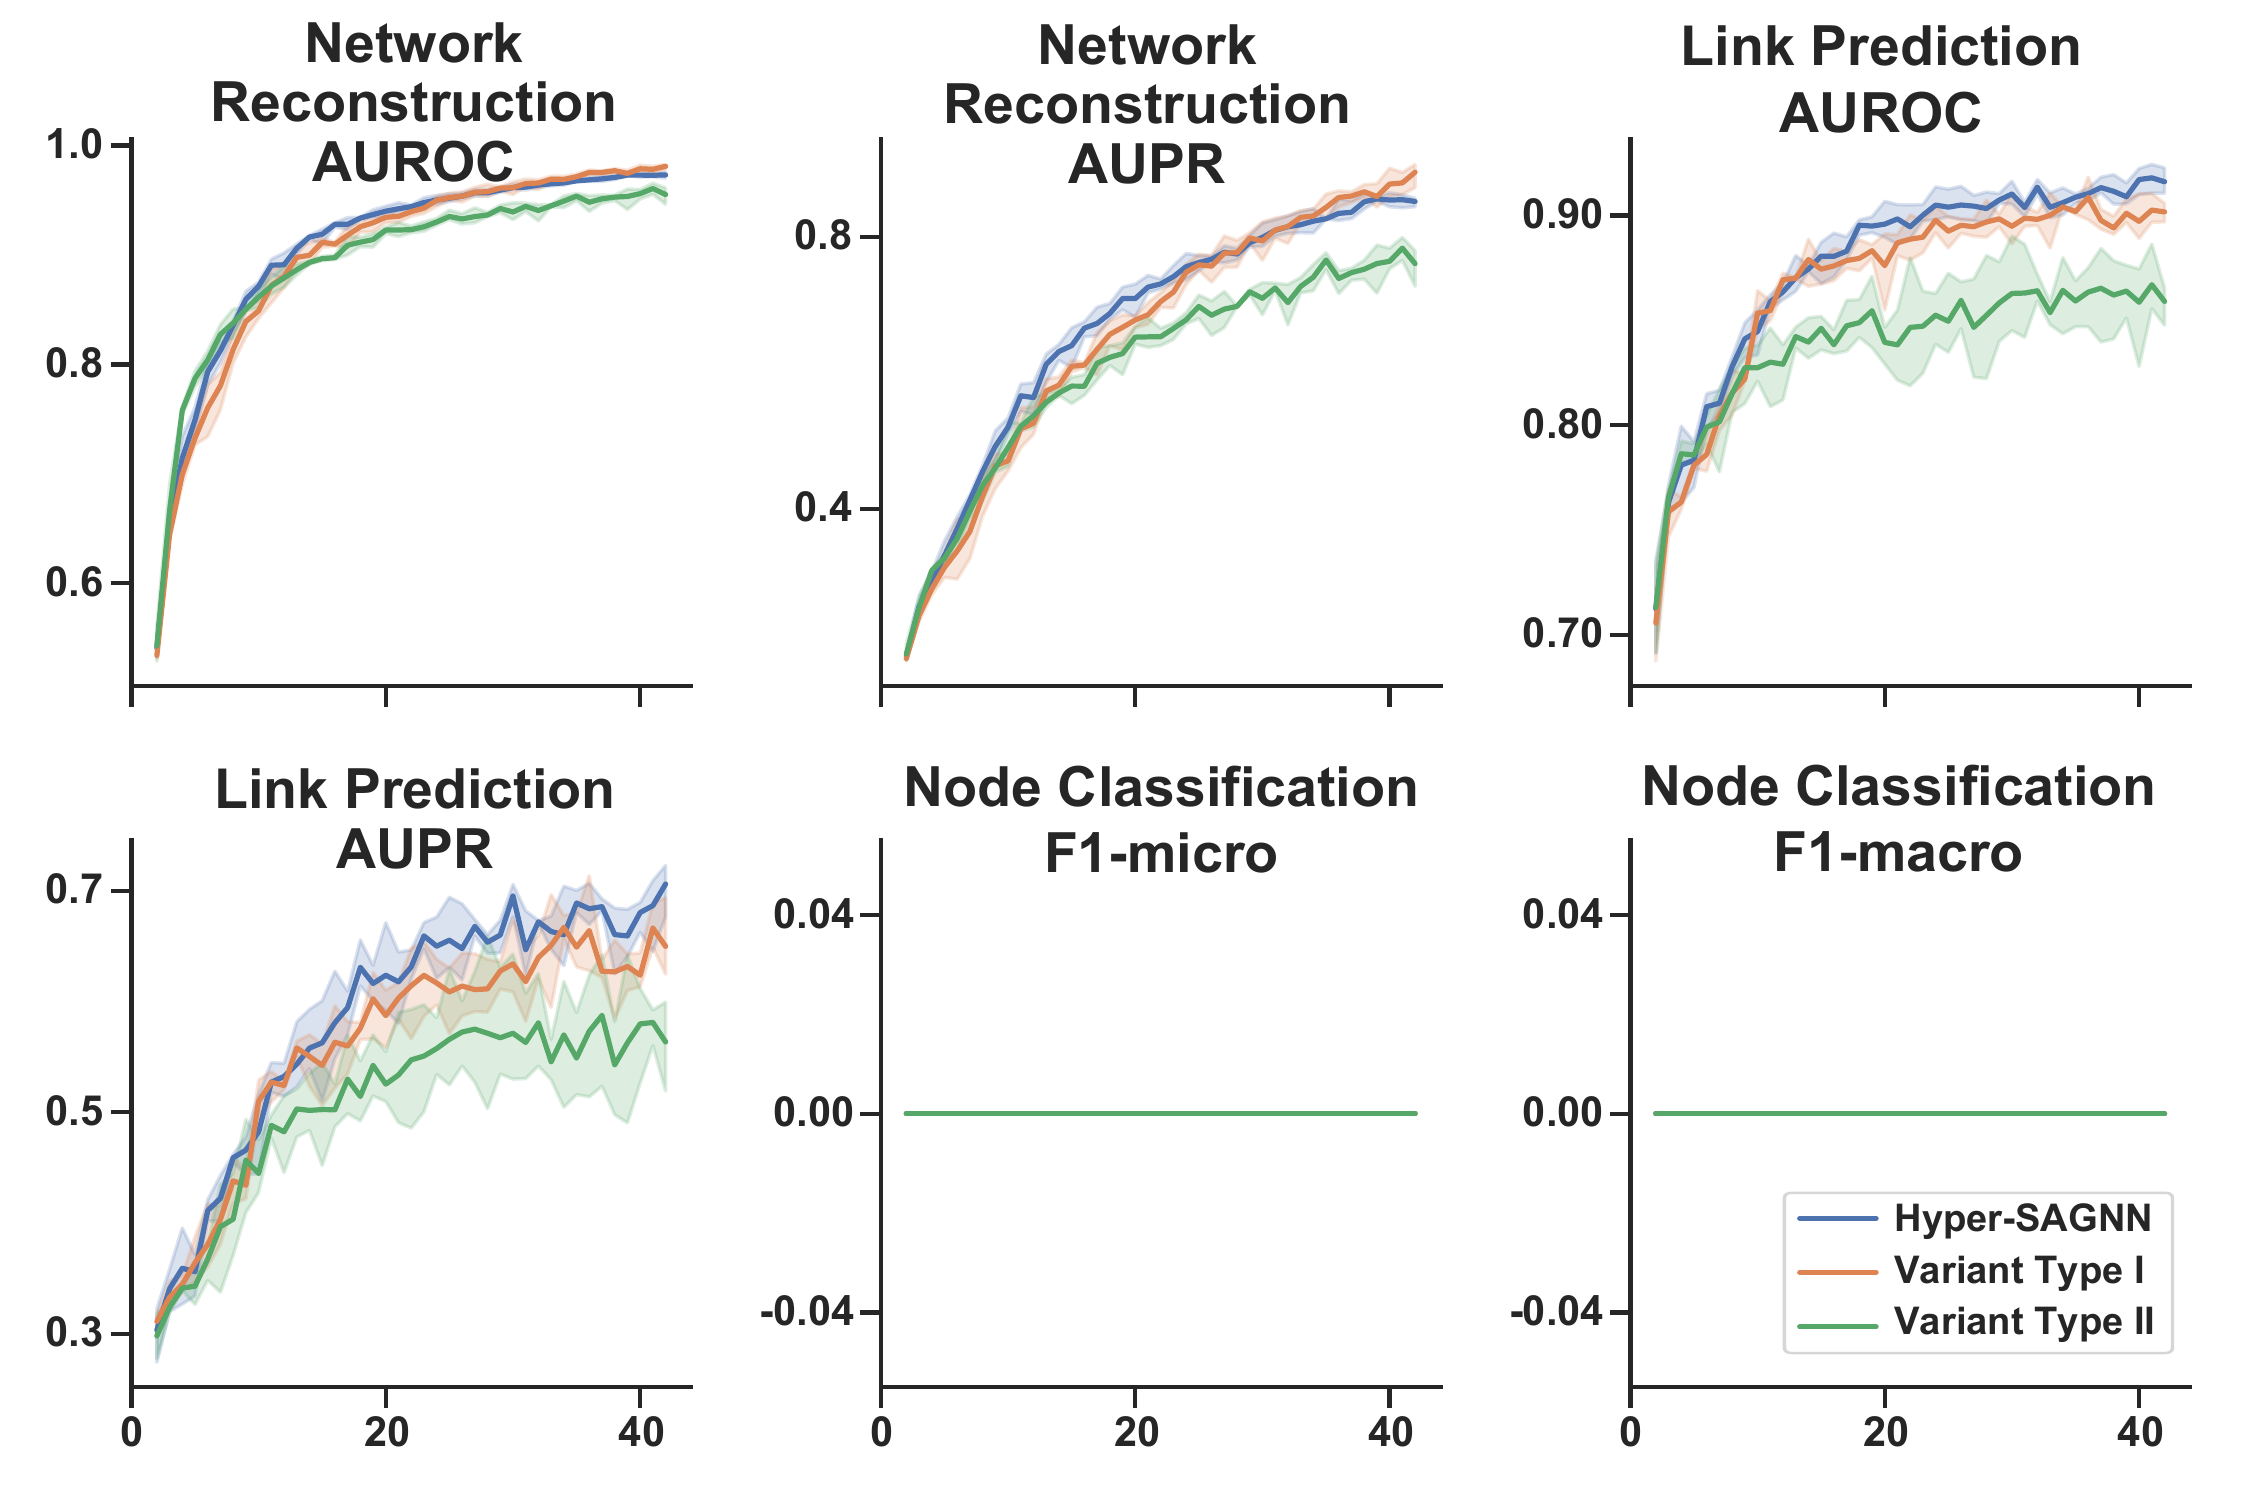}
    \caption{Performance Comparison of Our Model - Walk and Variant Type I, II(GPS)}
    \label{fig:perform_GPS1}
\end{figure}
\begin{figure}
    \centering
    \includegraphics[width = 0.75\textwidth]{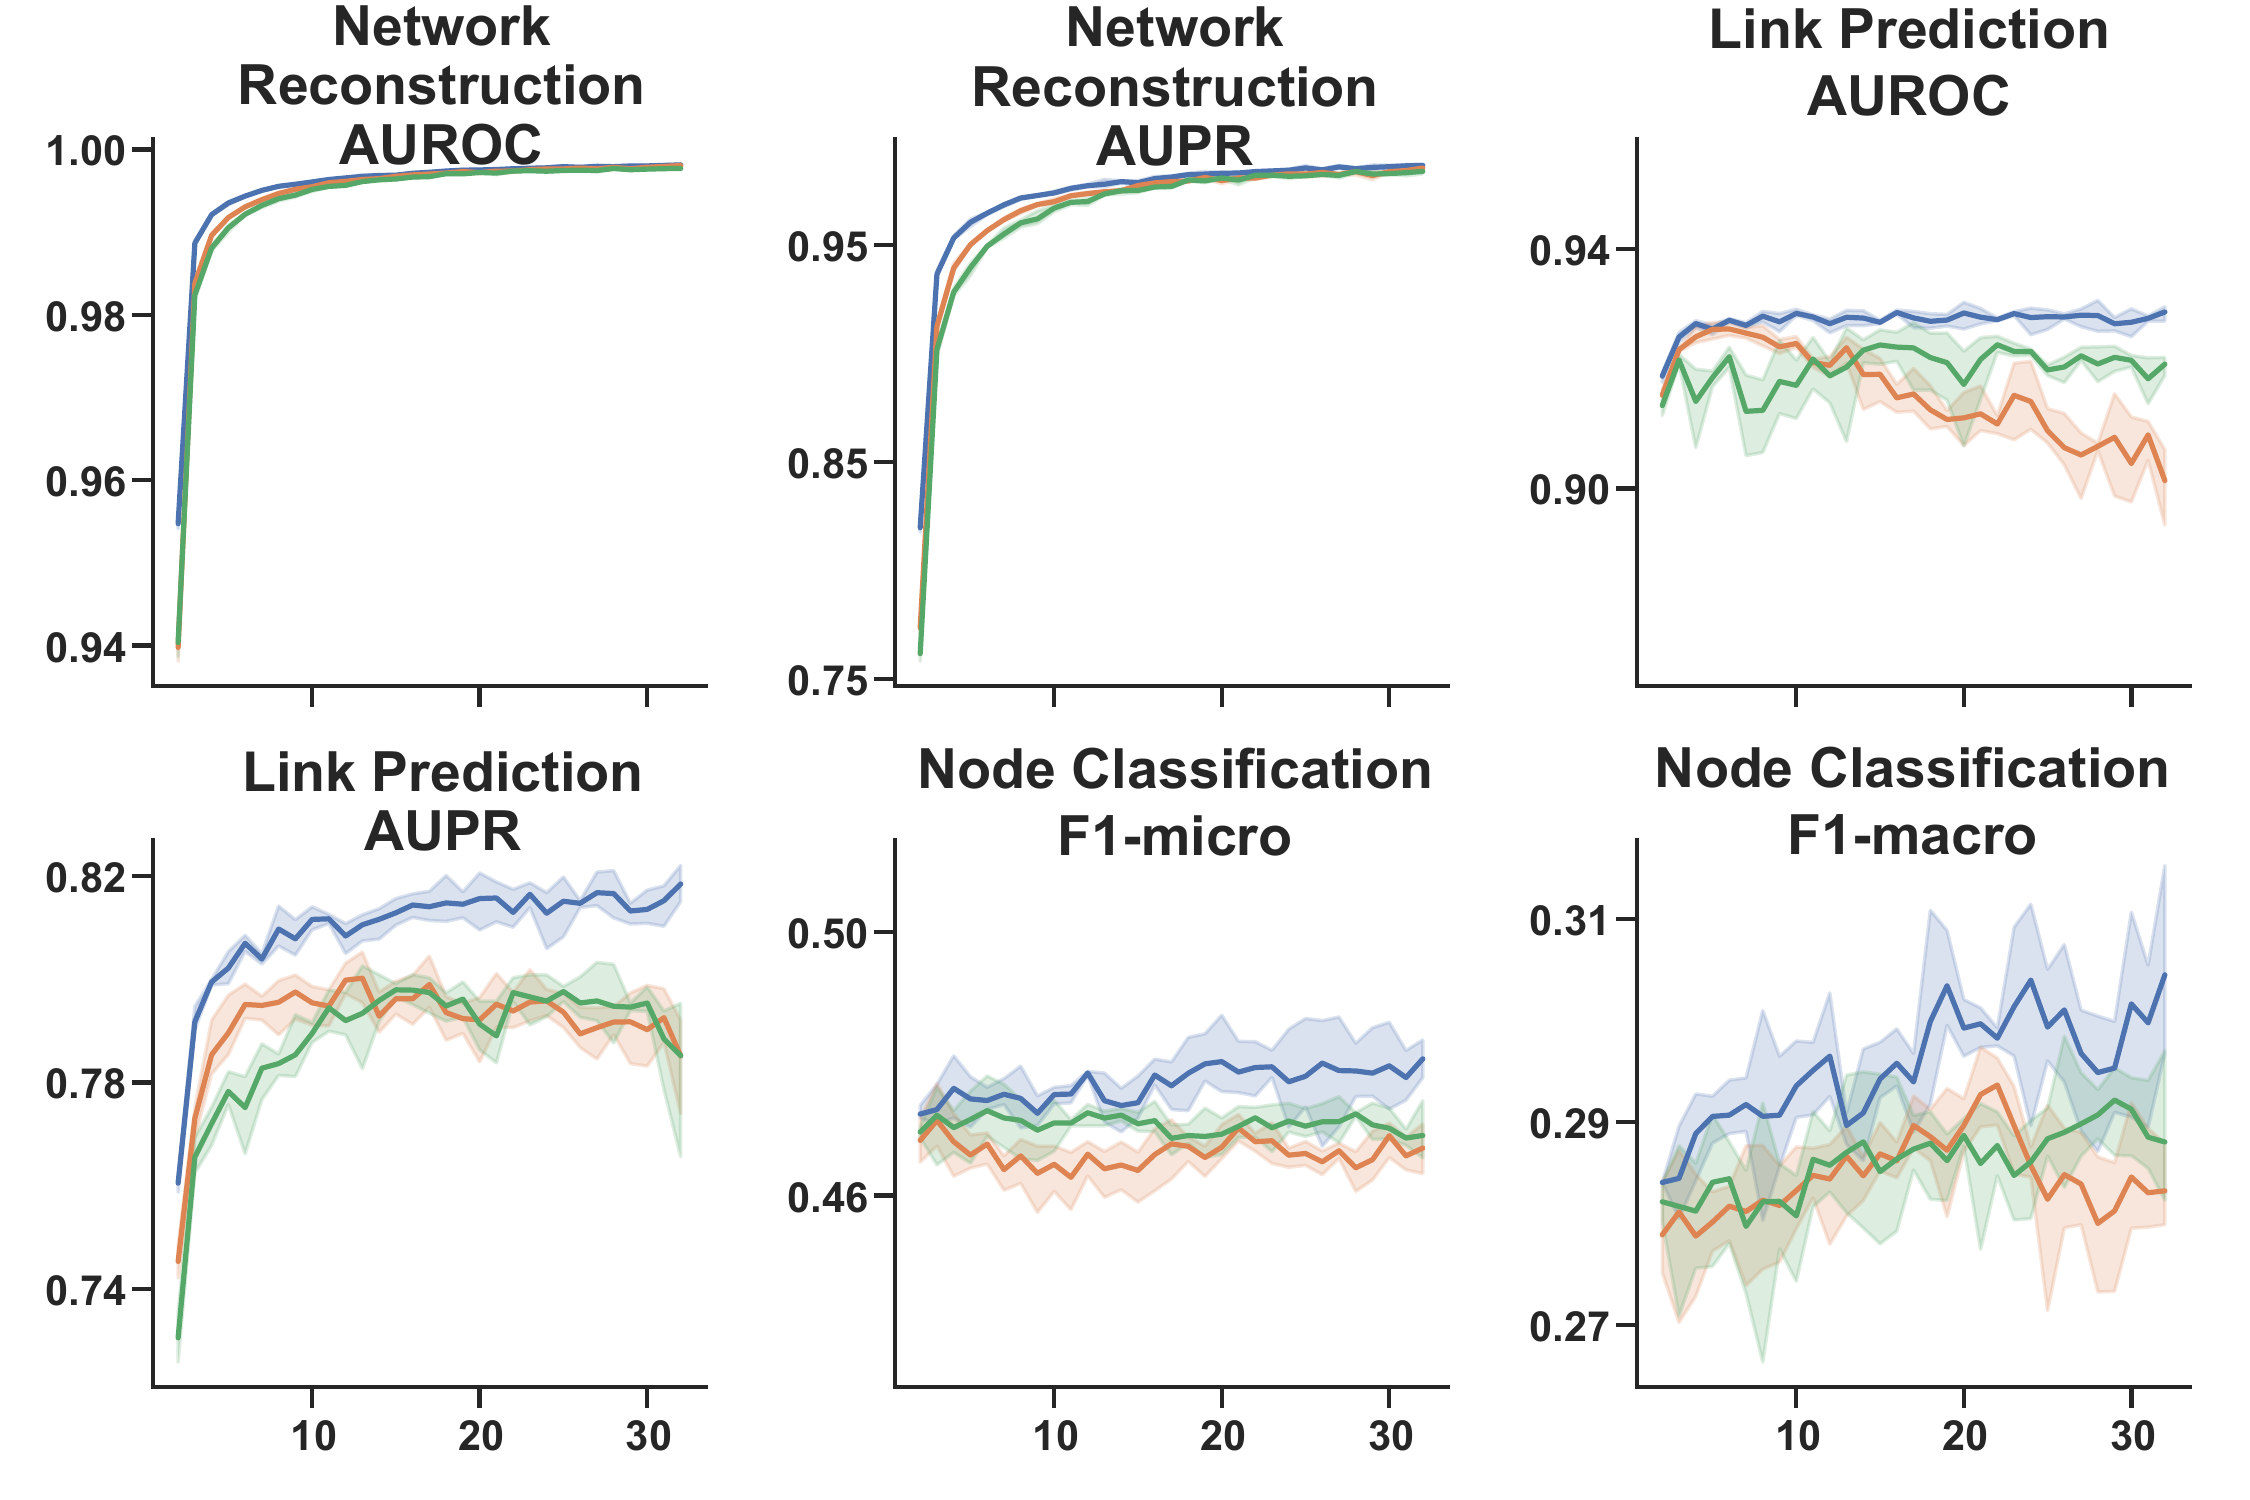}
    \caption{Performance Comparison of Our Model - Walk and Variant Type I, II(MovieLens)}
    \label{fig:perform_movie1}
\end{figure}
\begin{figure}
    \centering
    \includegraphics[width = 0.75\textwidth]{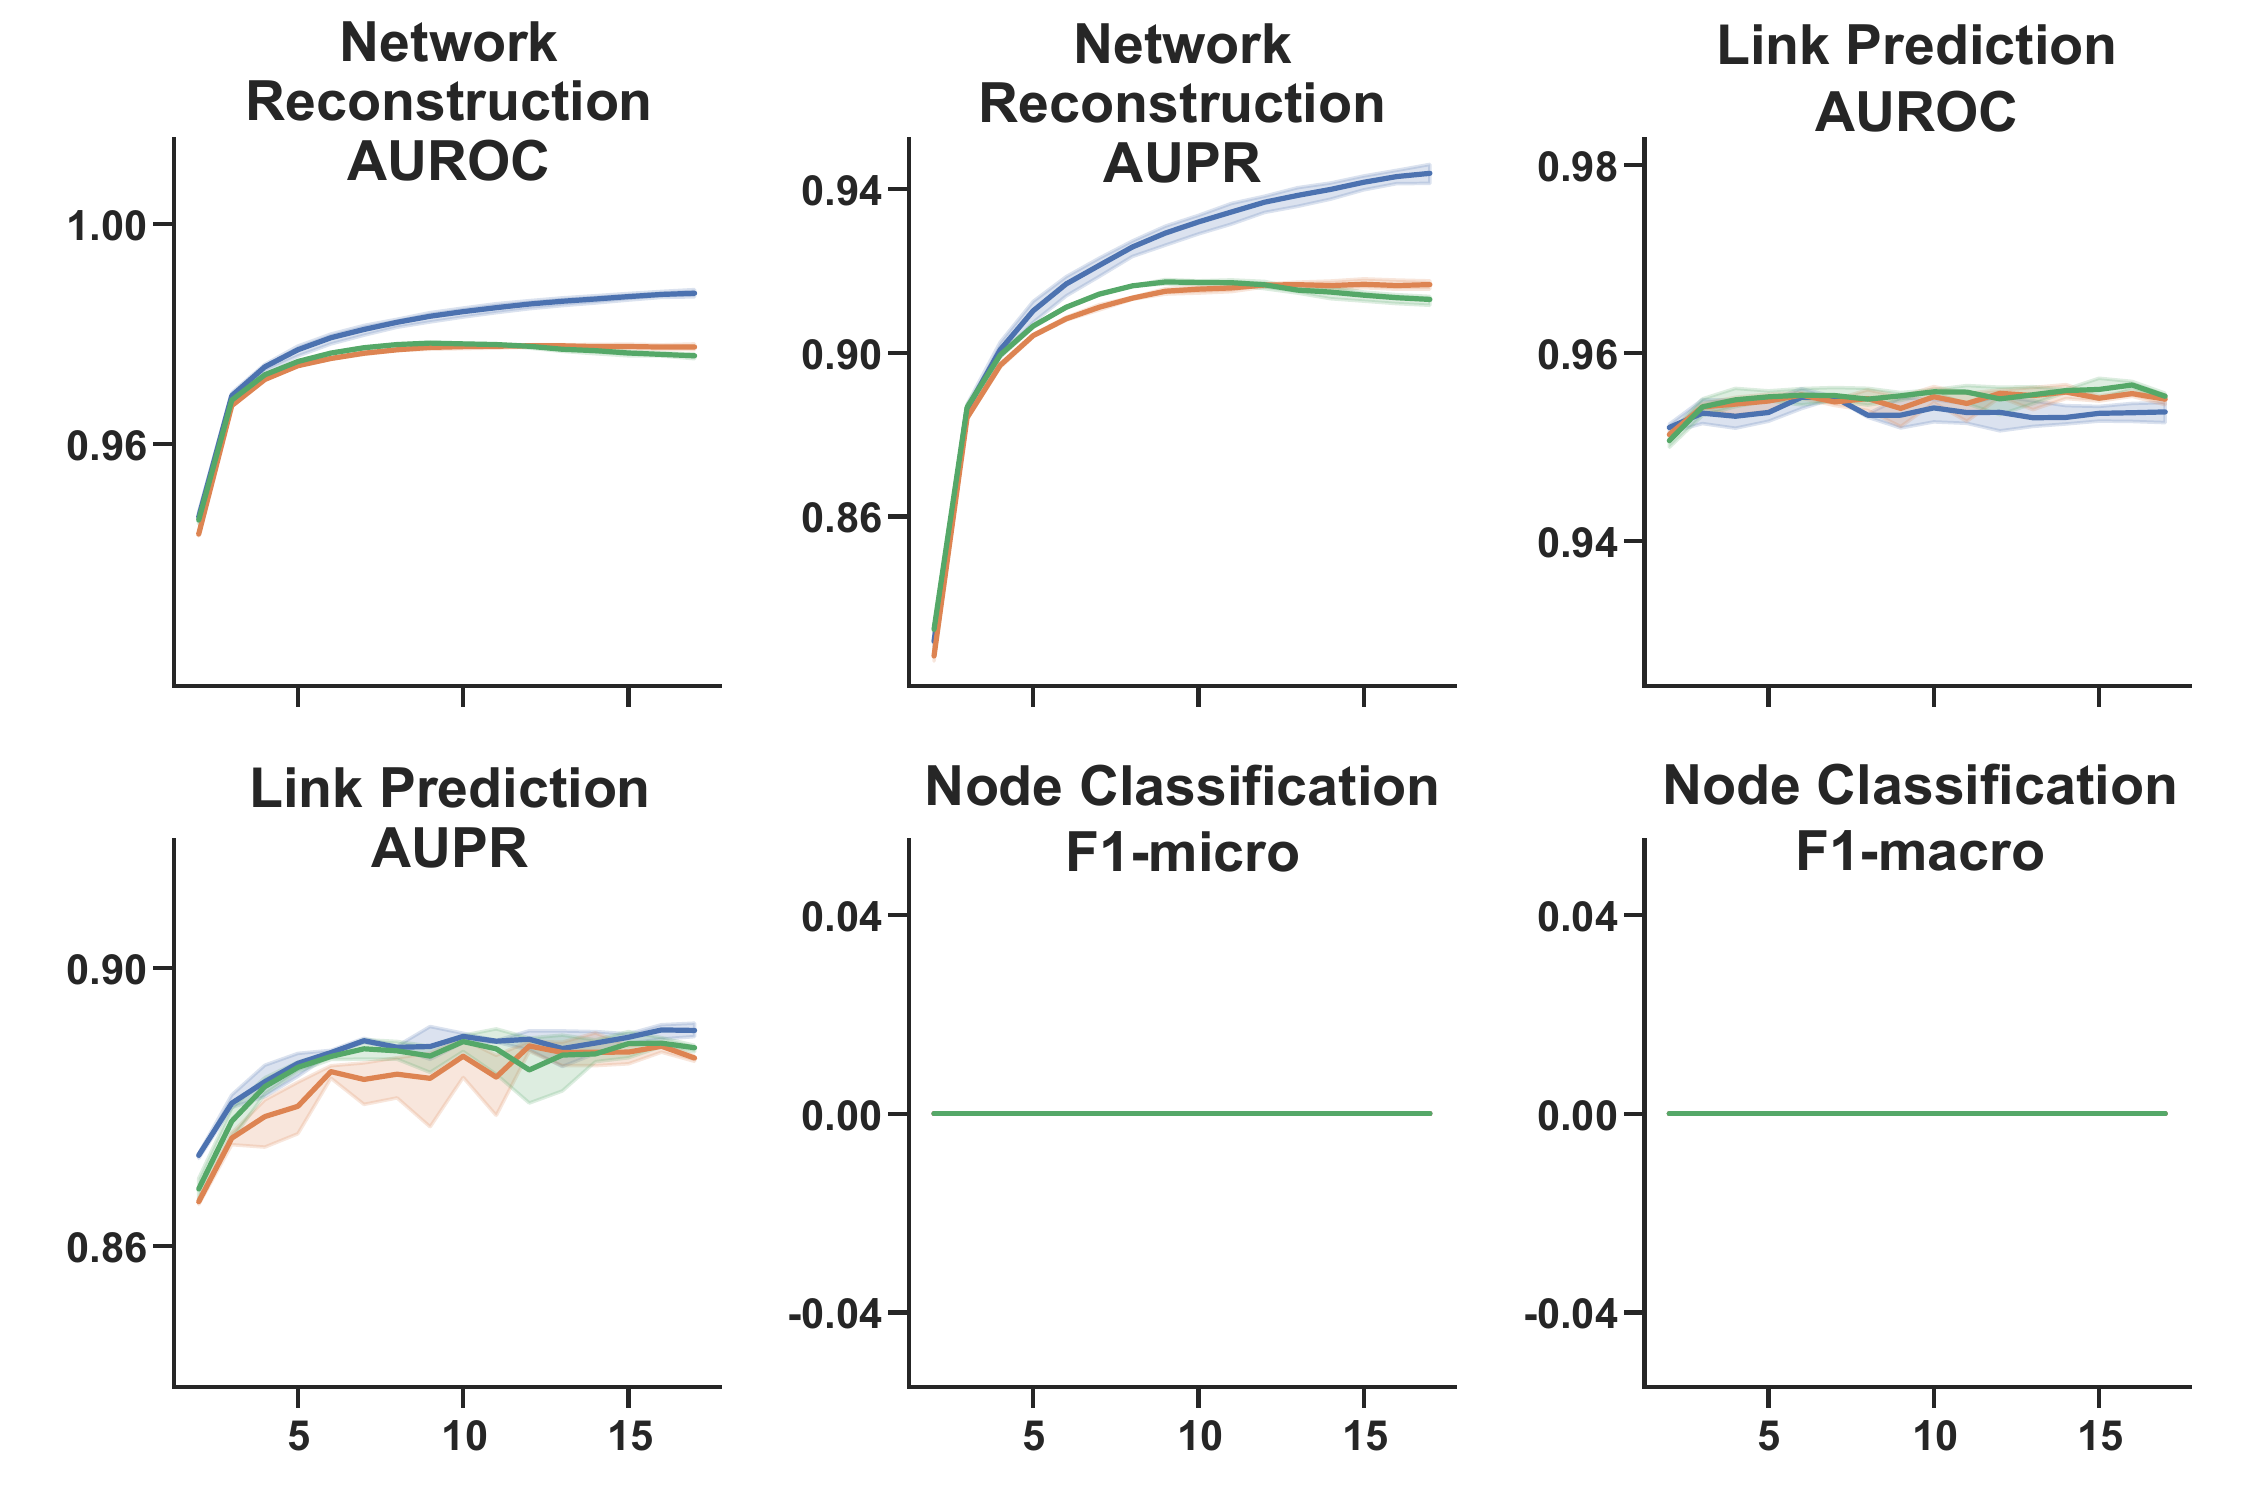}
    \caption{Performance Comparison of Our Model - Walk and Variant Type I, II(drug)}
    \label{fig:perform_drug1}
\end{figure}
\begin{figure}
    \centering
    \includegraphics[width = 0.75\textwidth]{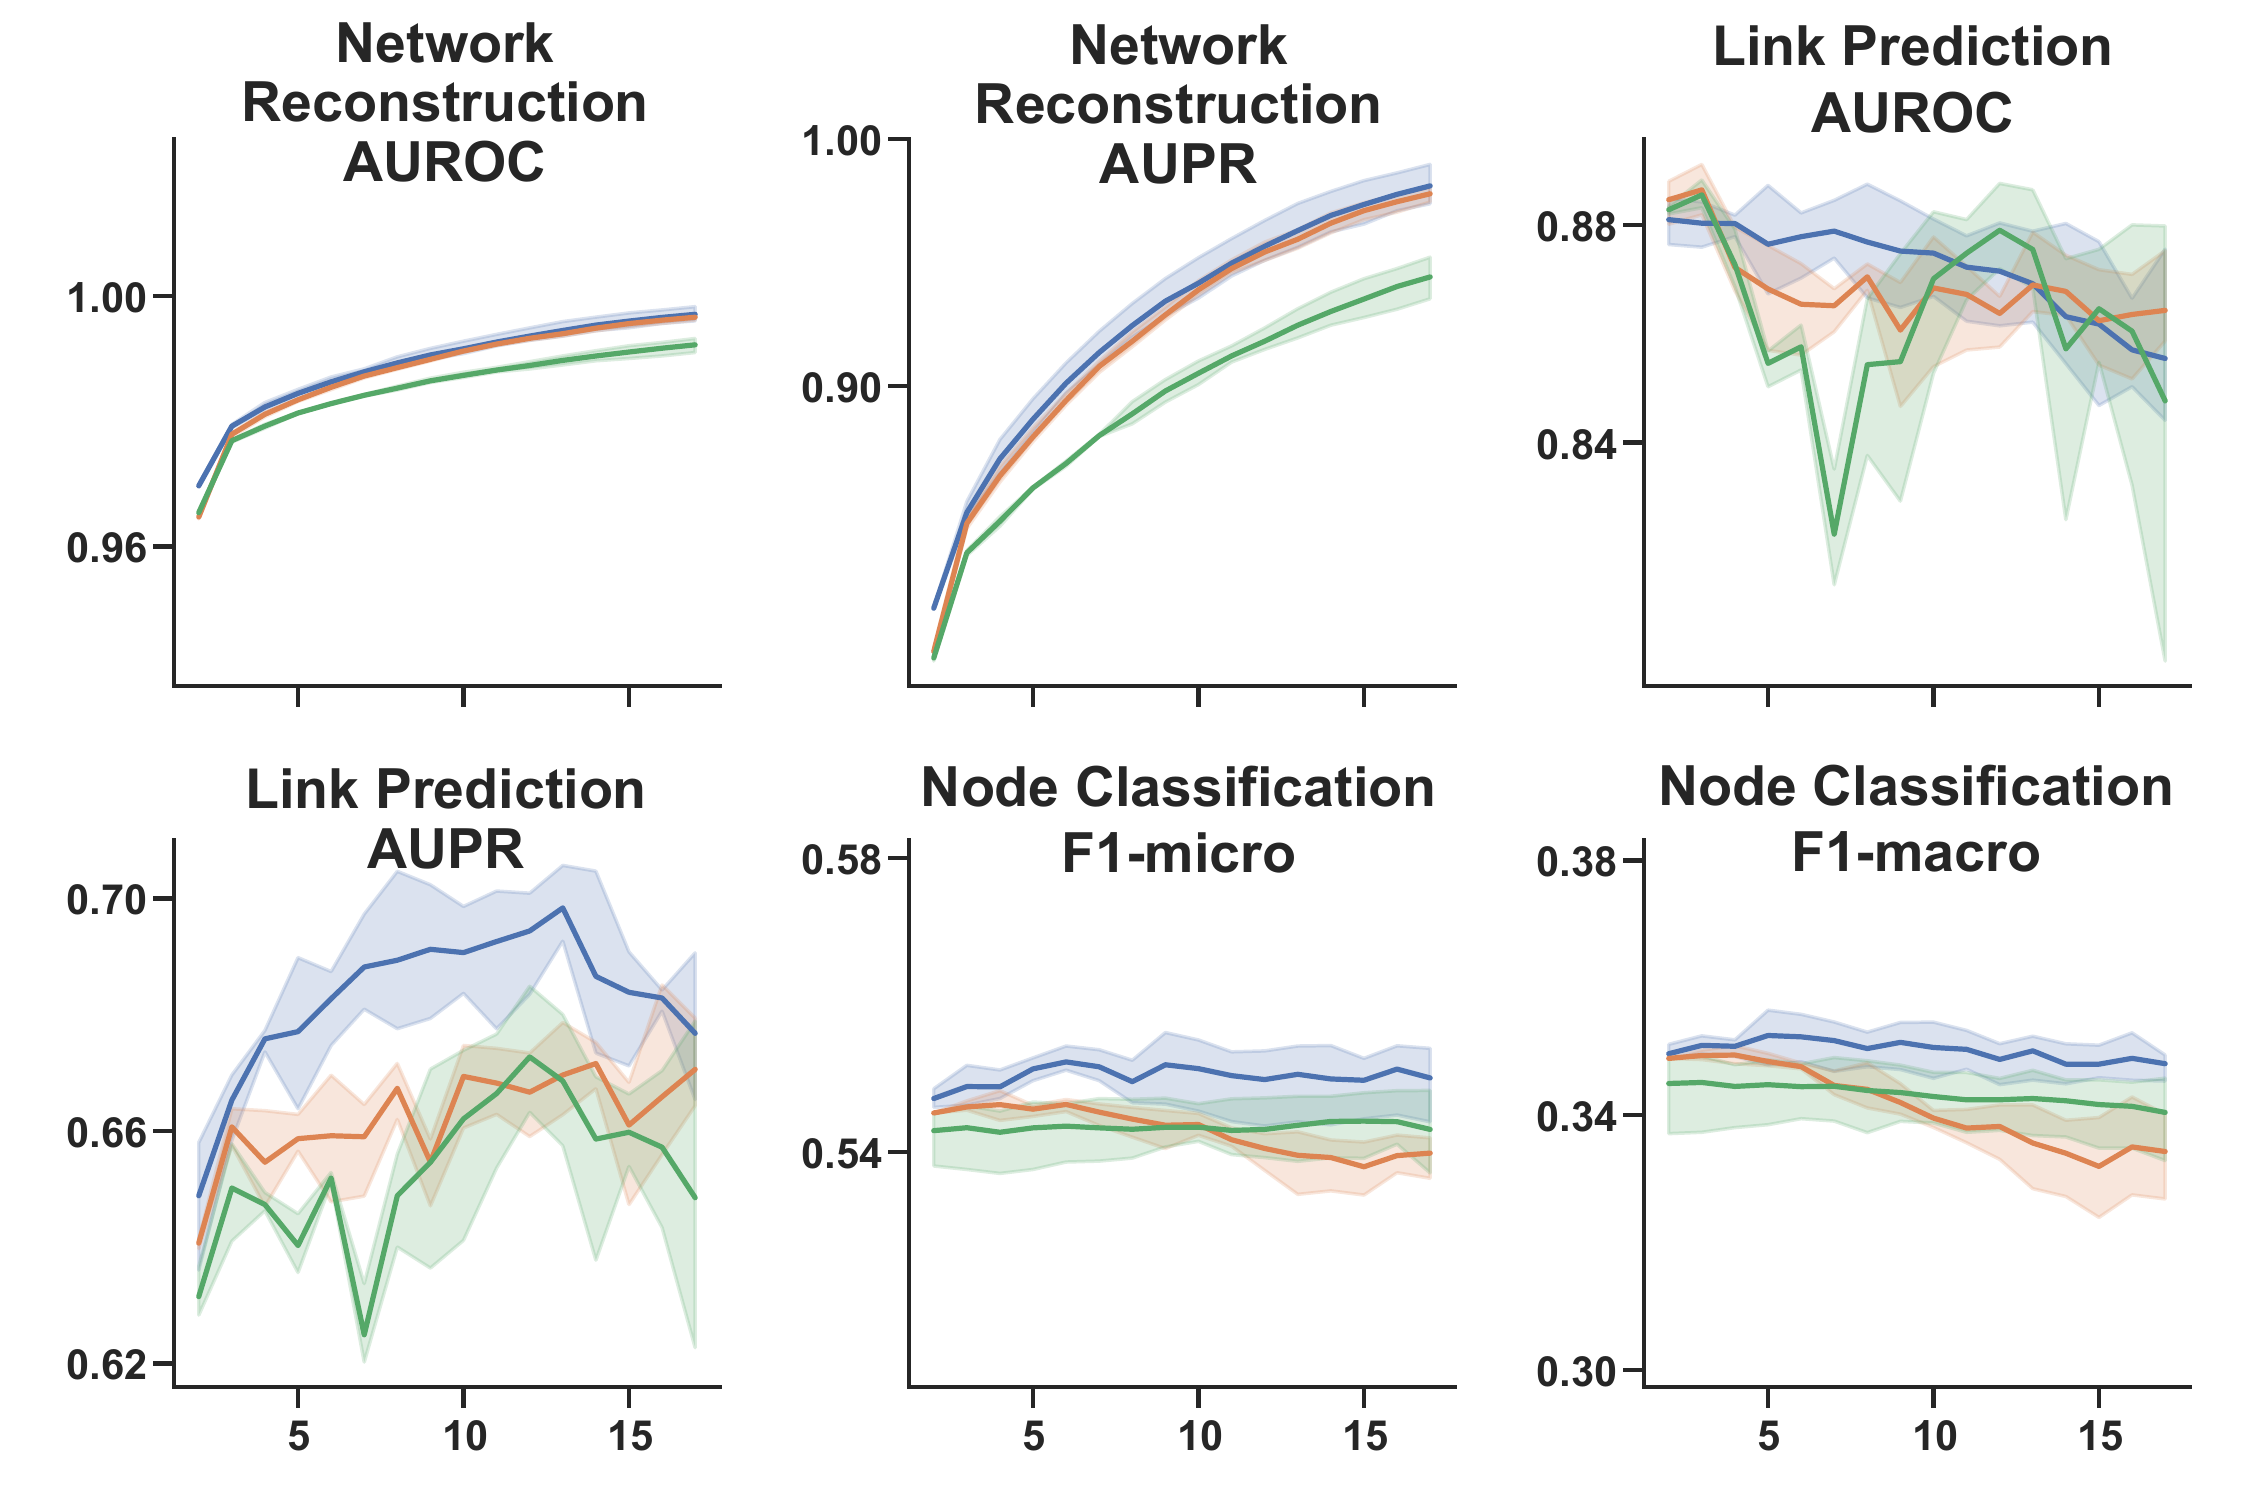}
    \caption{Performance Comparison of Our Model - Walk and Variant Type I, II(wordnet)}
    \label{fig:perform_wordnet1}
\end{figure}
\begin{figure}
    \centering
    \includegraphics[width = 0.75\textwidth]{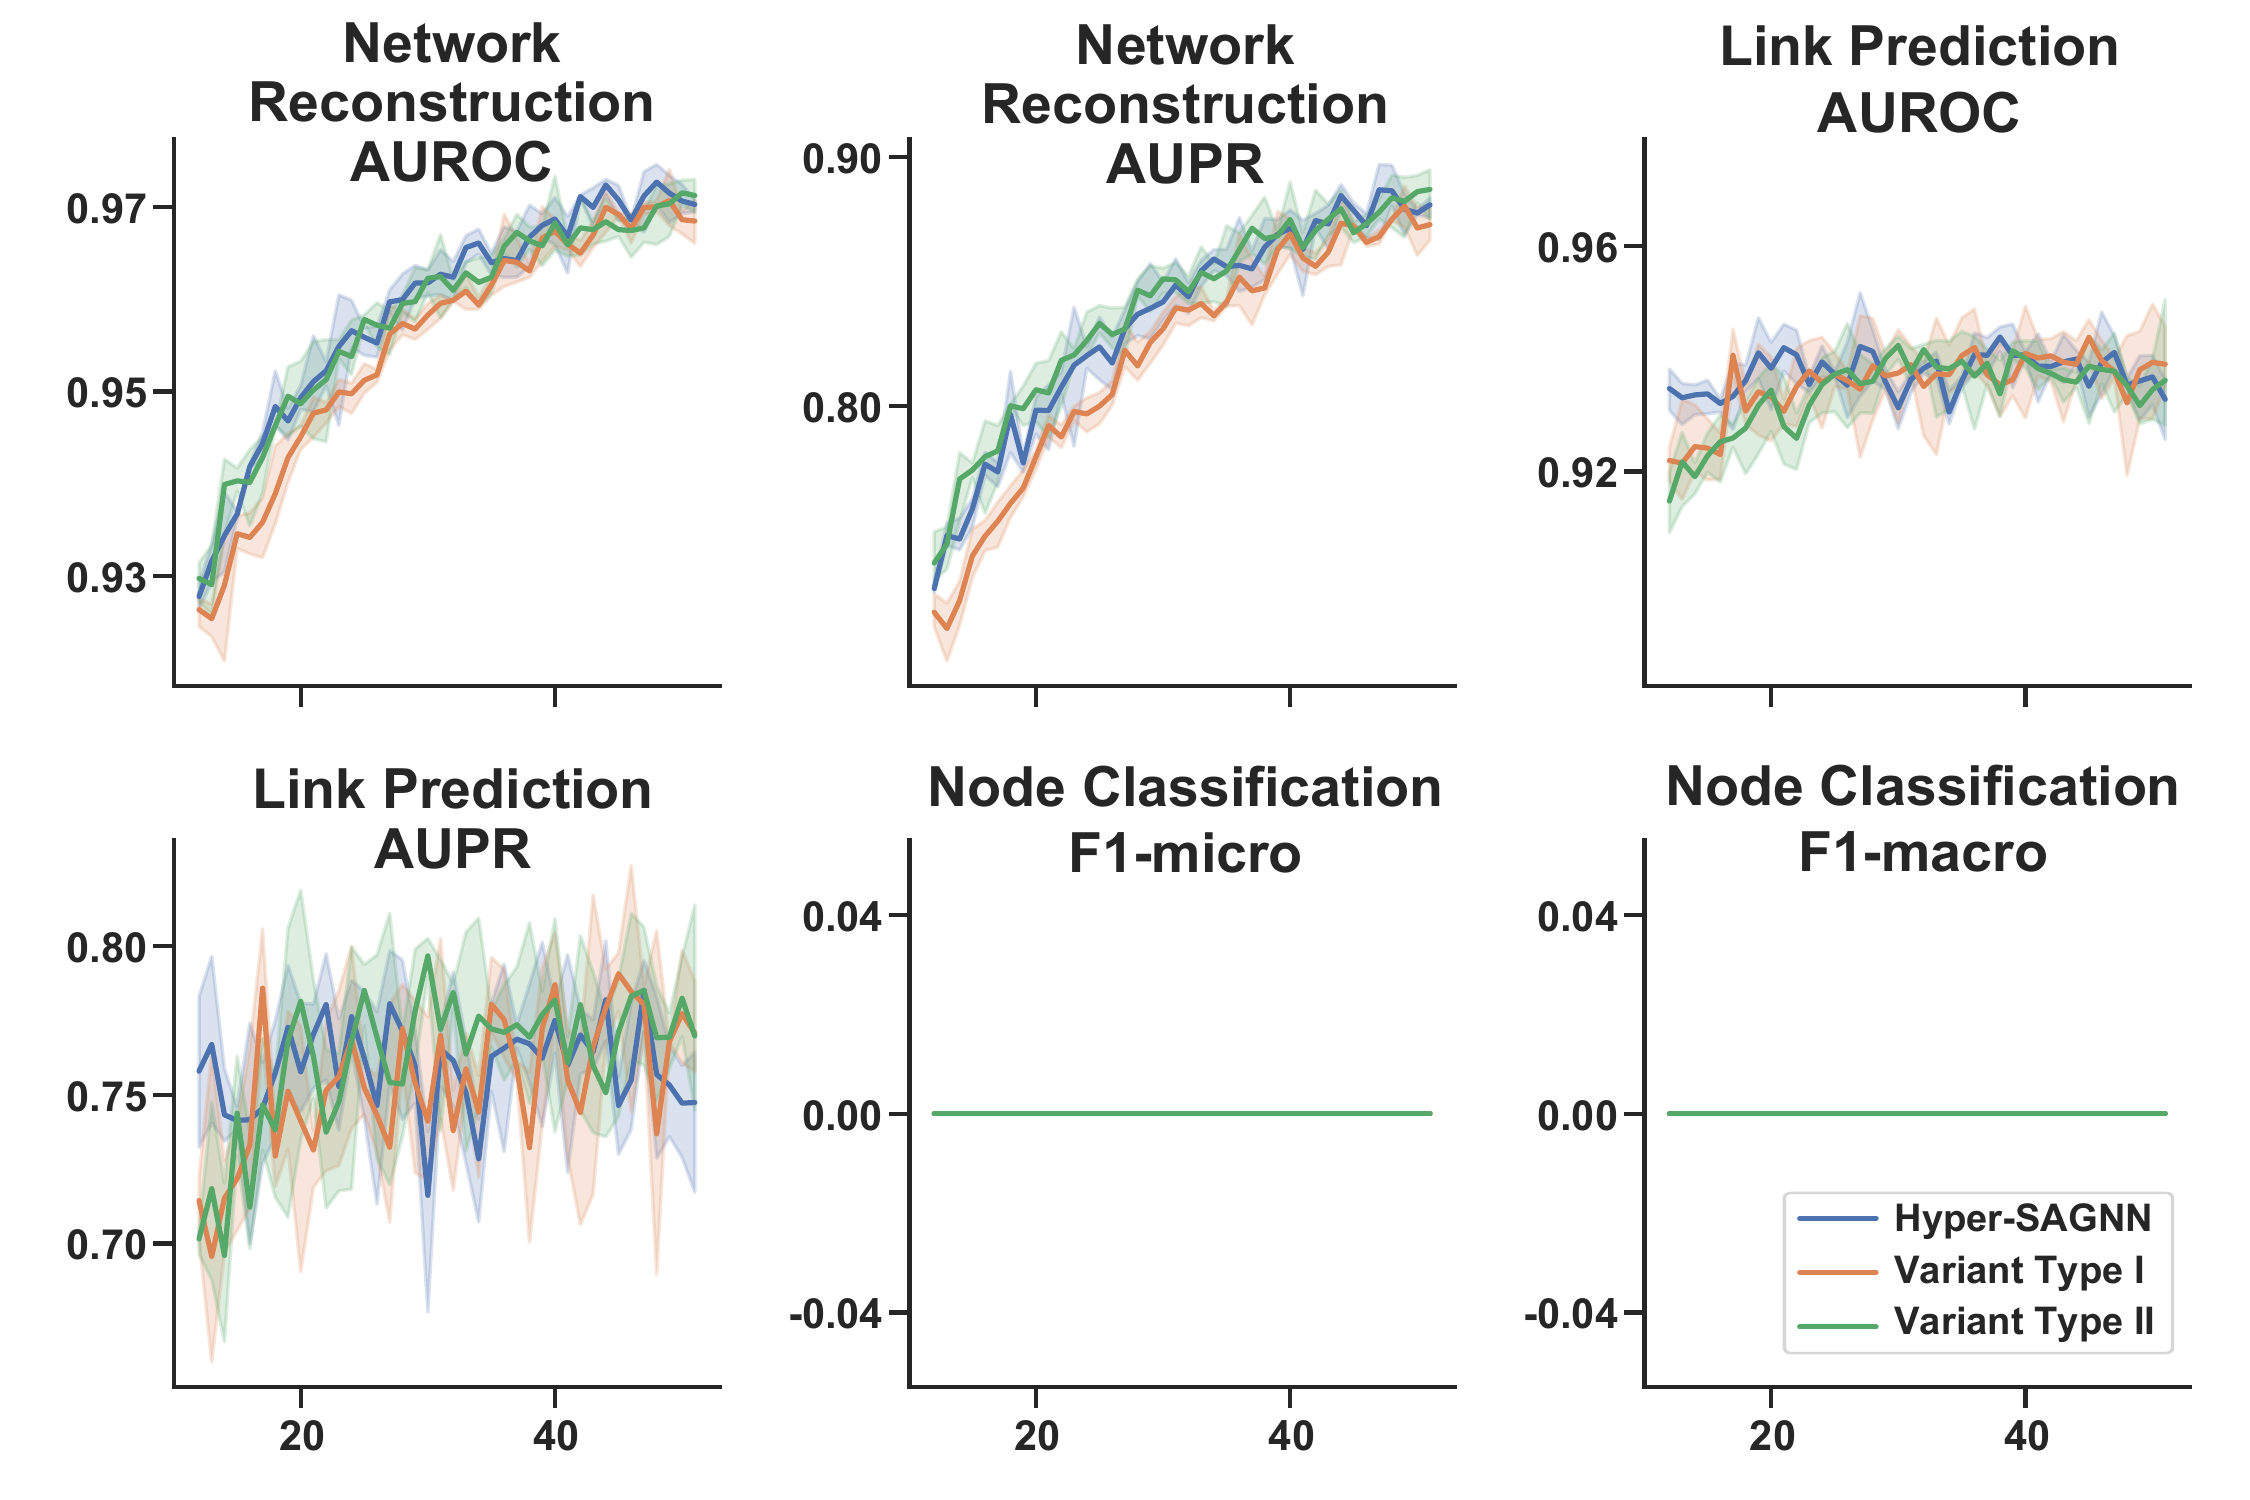}
    \caption{Performance Comparison of Our Model - Encoder and Variant Type I, II(GPS)}
    \label{fig:perform_GPS2}
\end{figure}
\begin{figure}
    \centering
    \includegraphics[width = 0.75\textwidth]{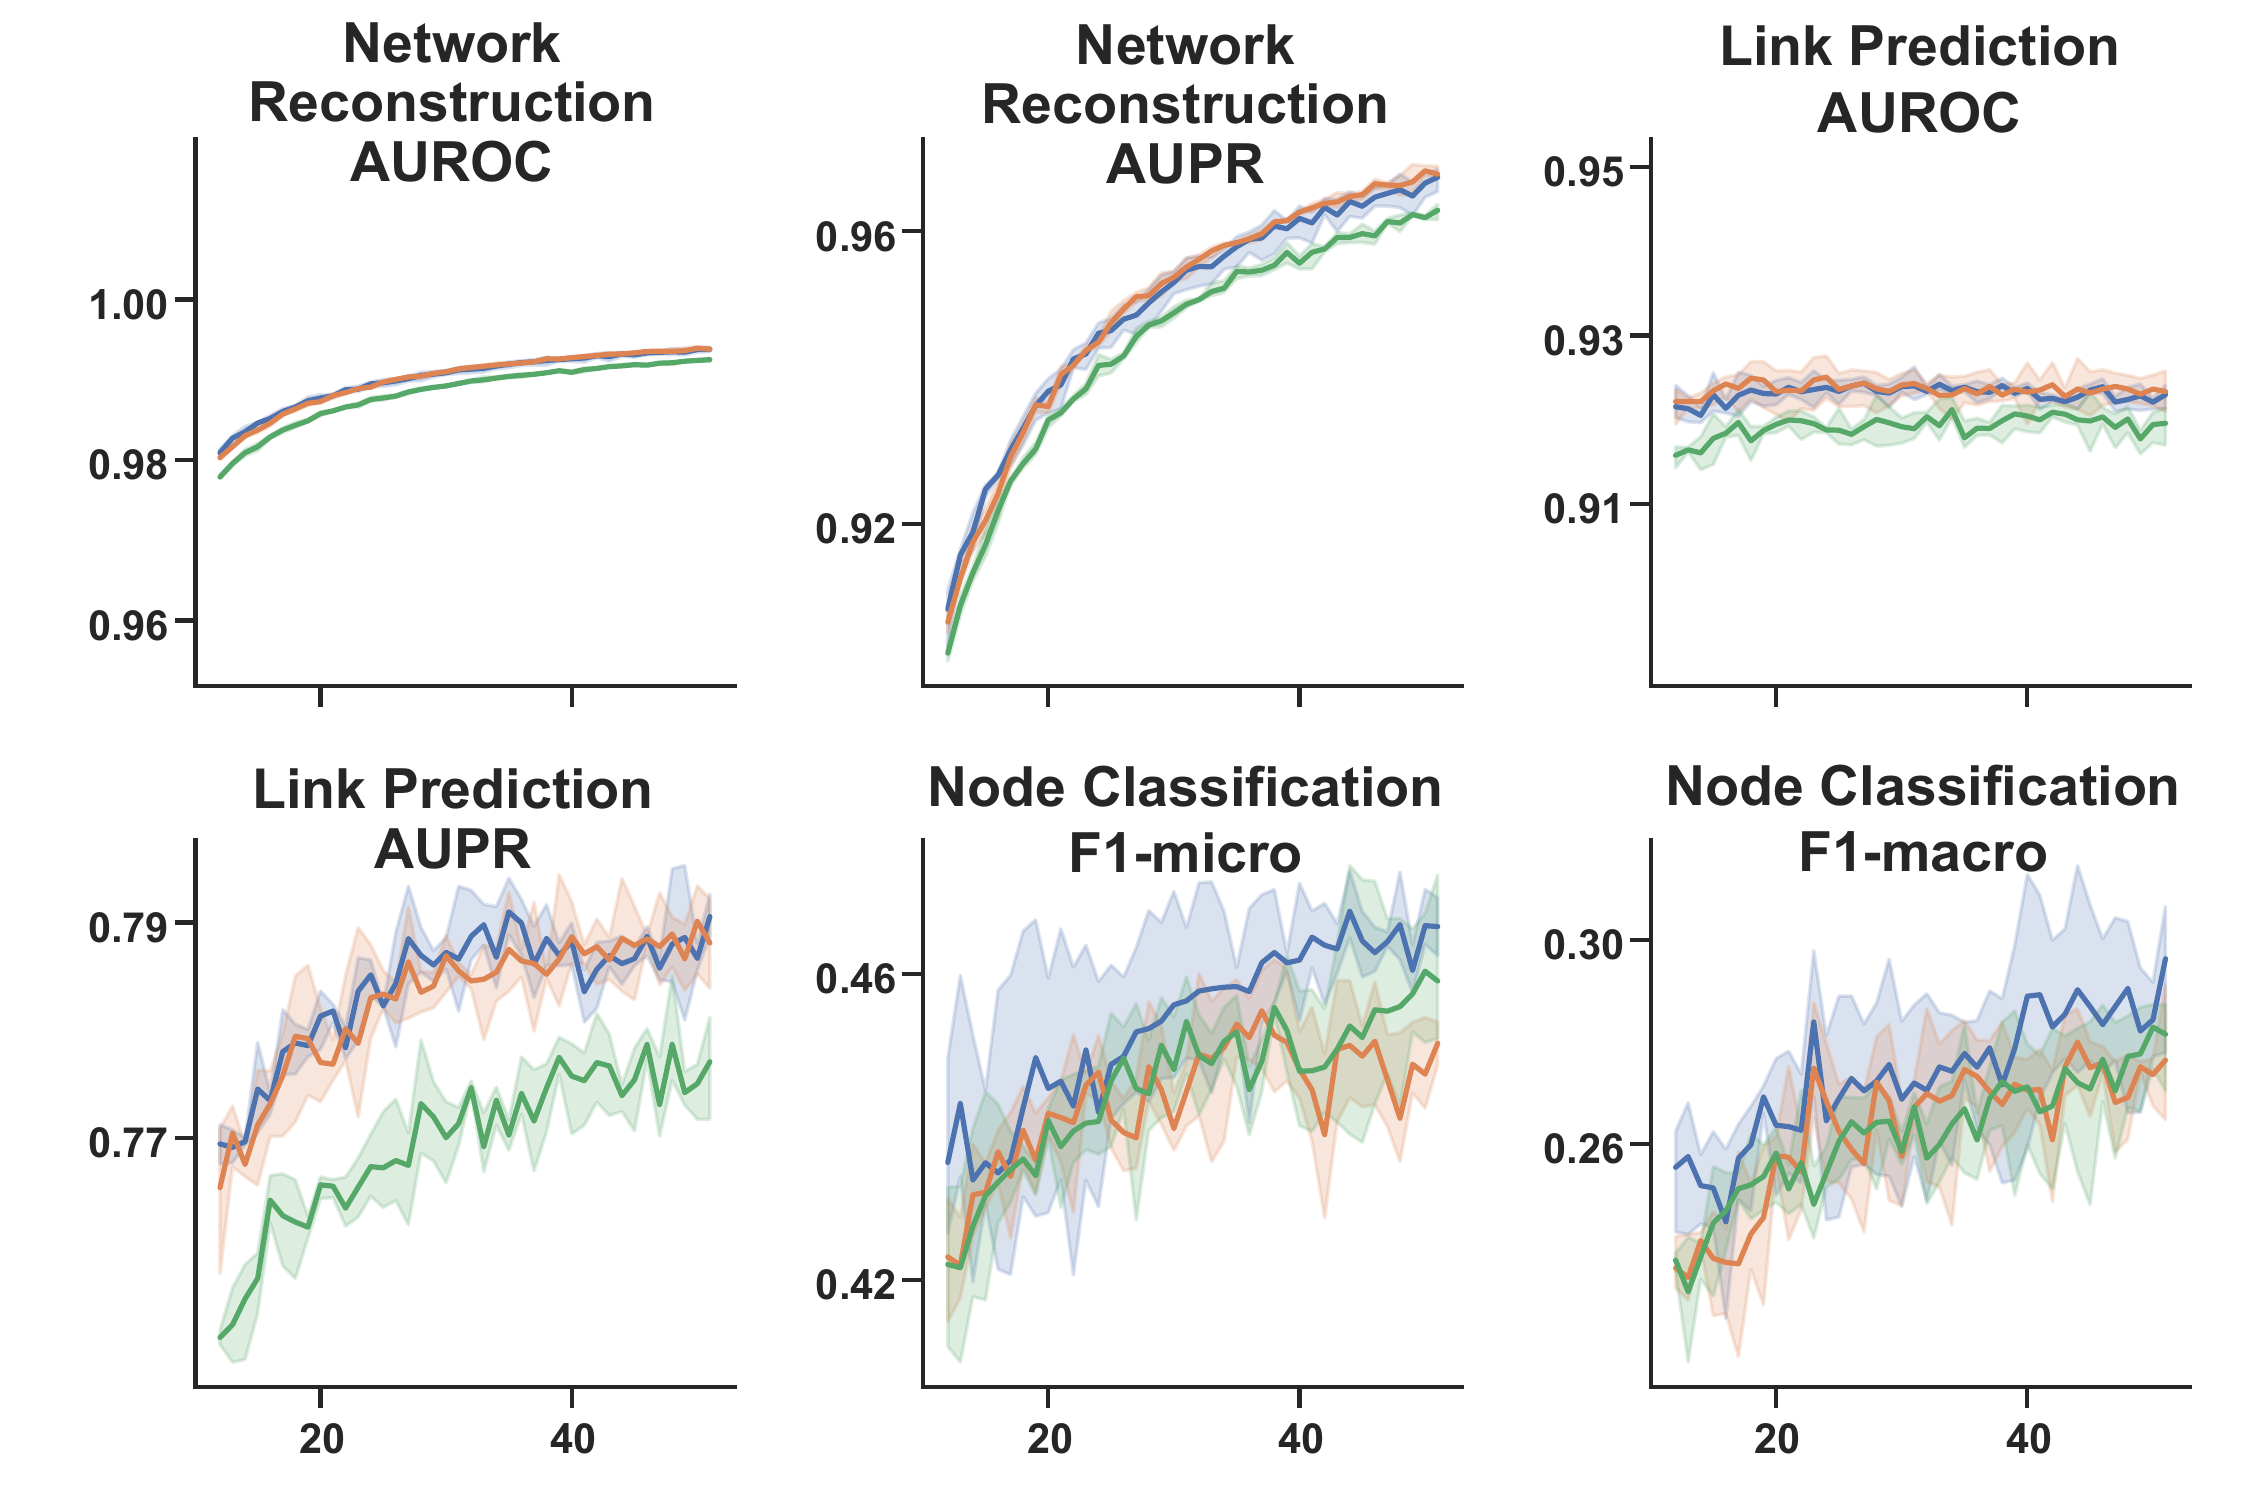}
    \caption{Performance Comparison of Our Model - Encoder and Variant Type I, II(MovieLens)}
    \label{fig:perform_movie2}
\end{figure}
\begin{figure}
    \centering
    \includegraphics[width = 0.75\textwidth]{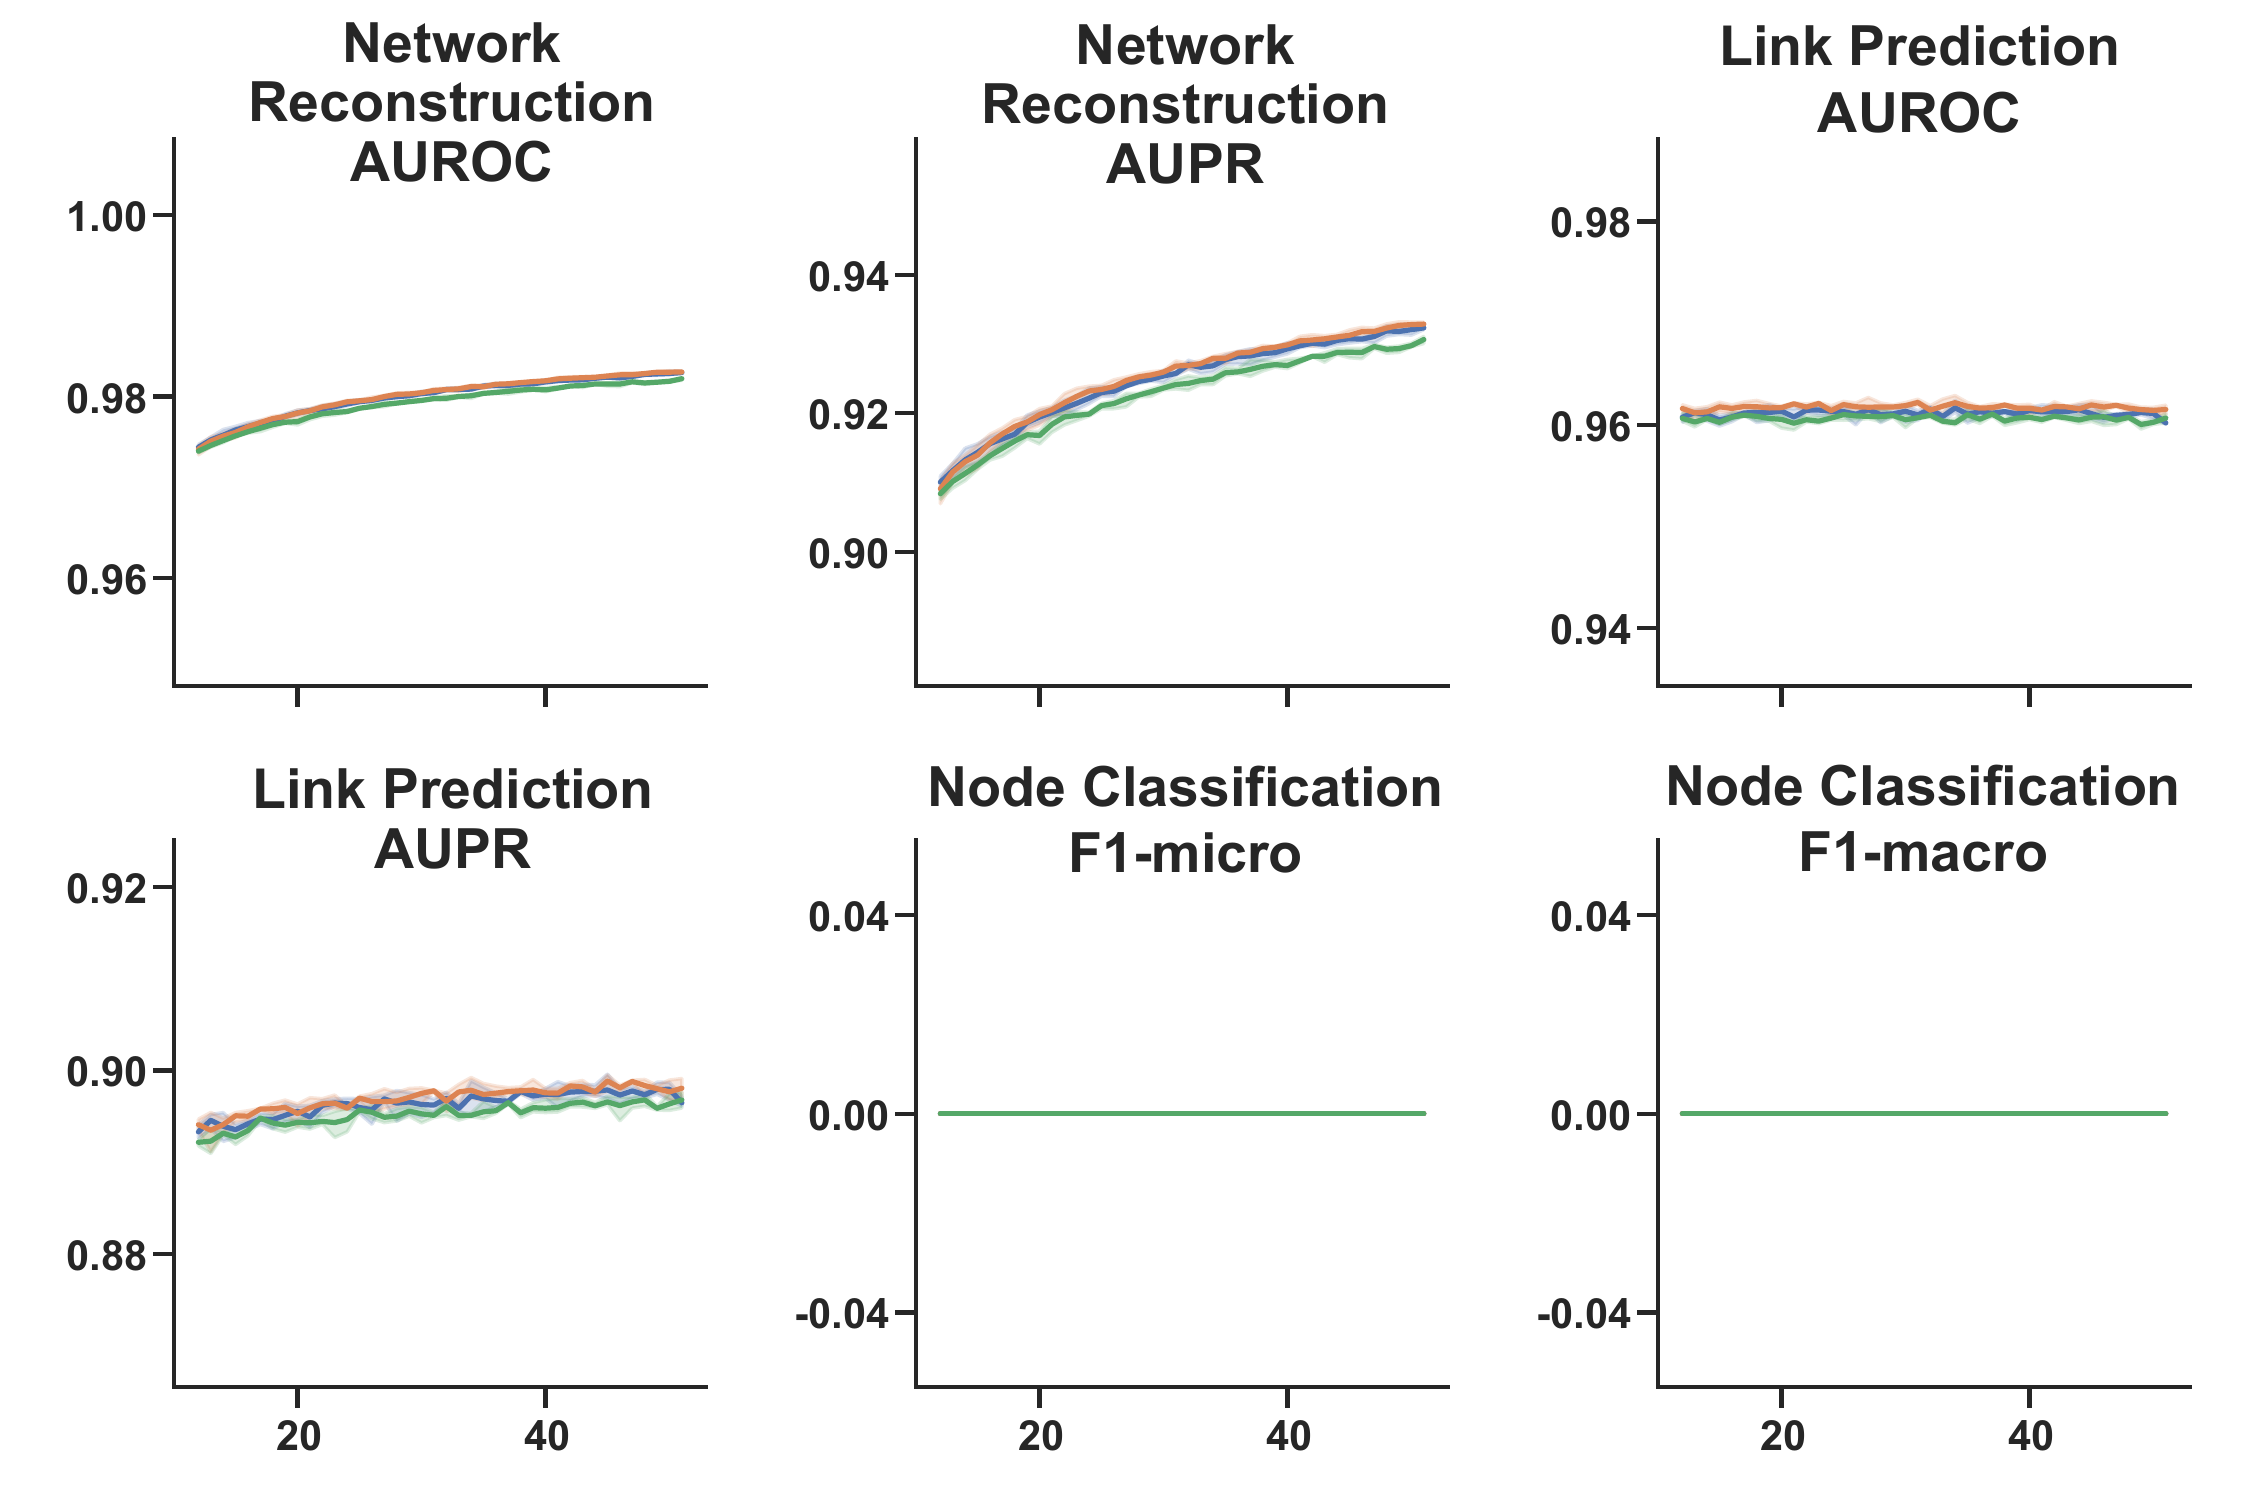}
    \caption{Performance Comparison of Our Model - Encoder and Variant Type I, II(drug)}
    \label{fig:perform_drug2}
\end{figure}
\begin{figure}
    \centering
    \includegraphics[width = 0.75\textwidth]{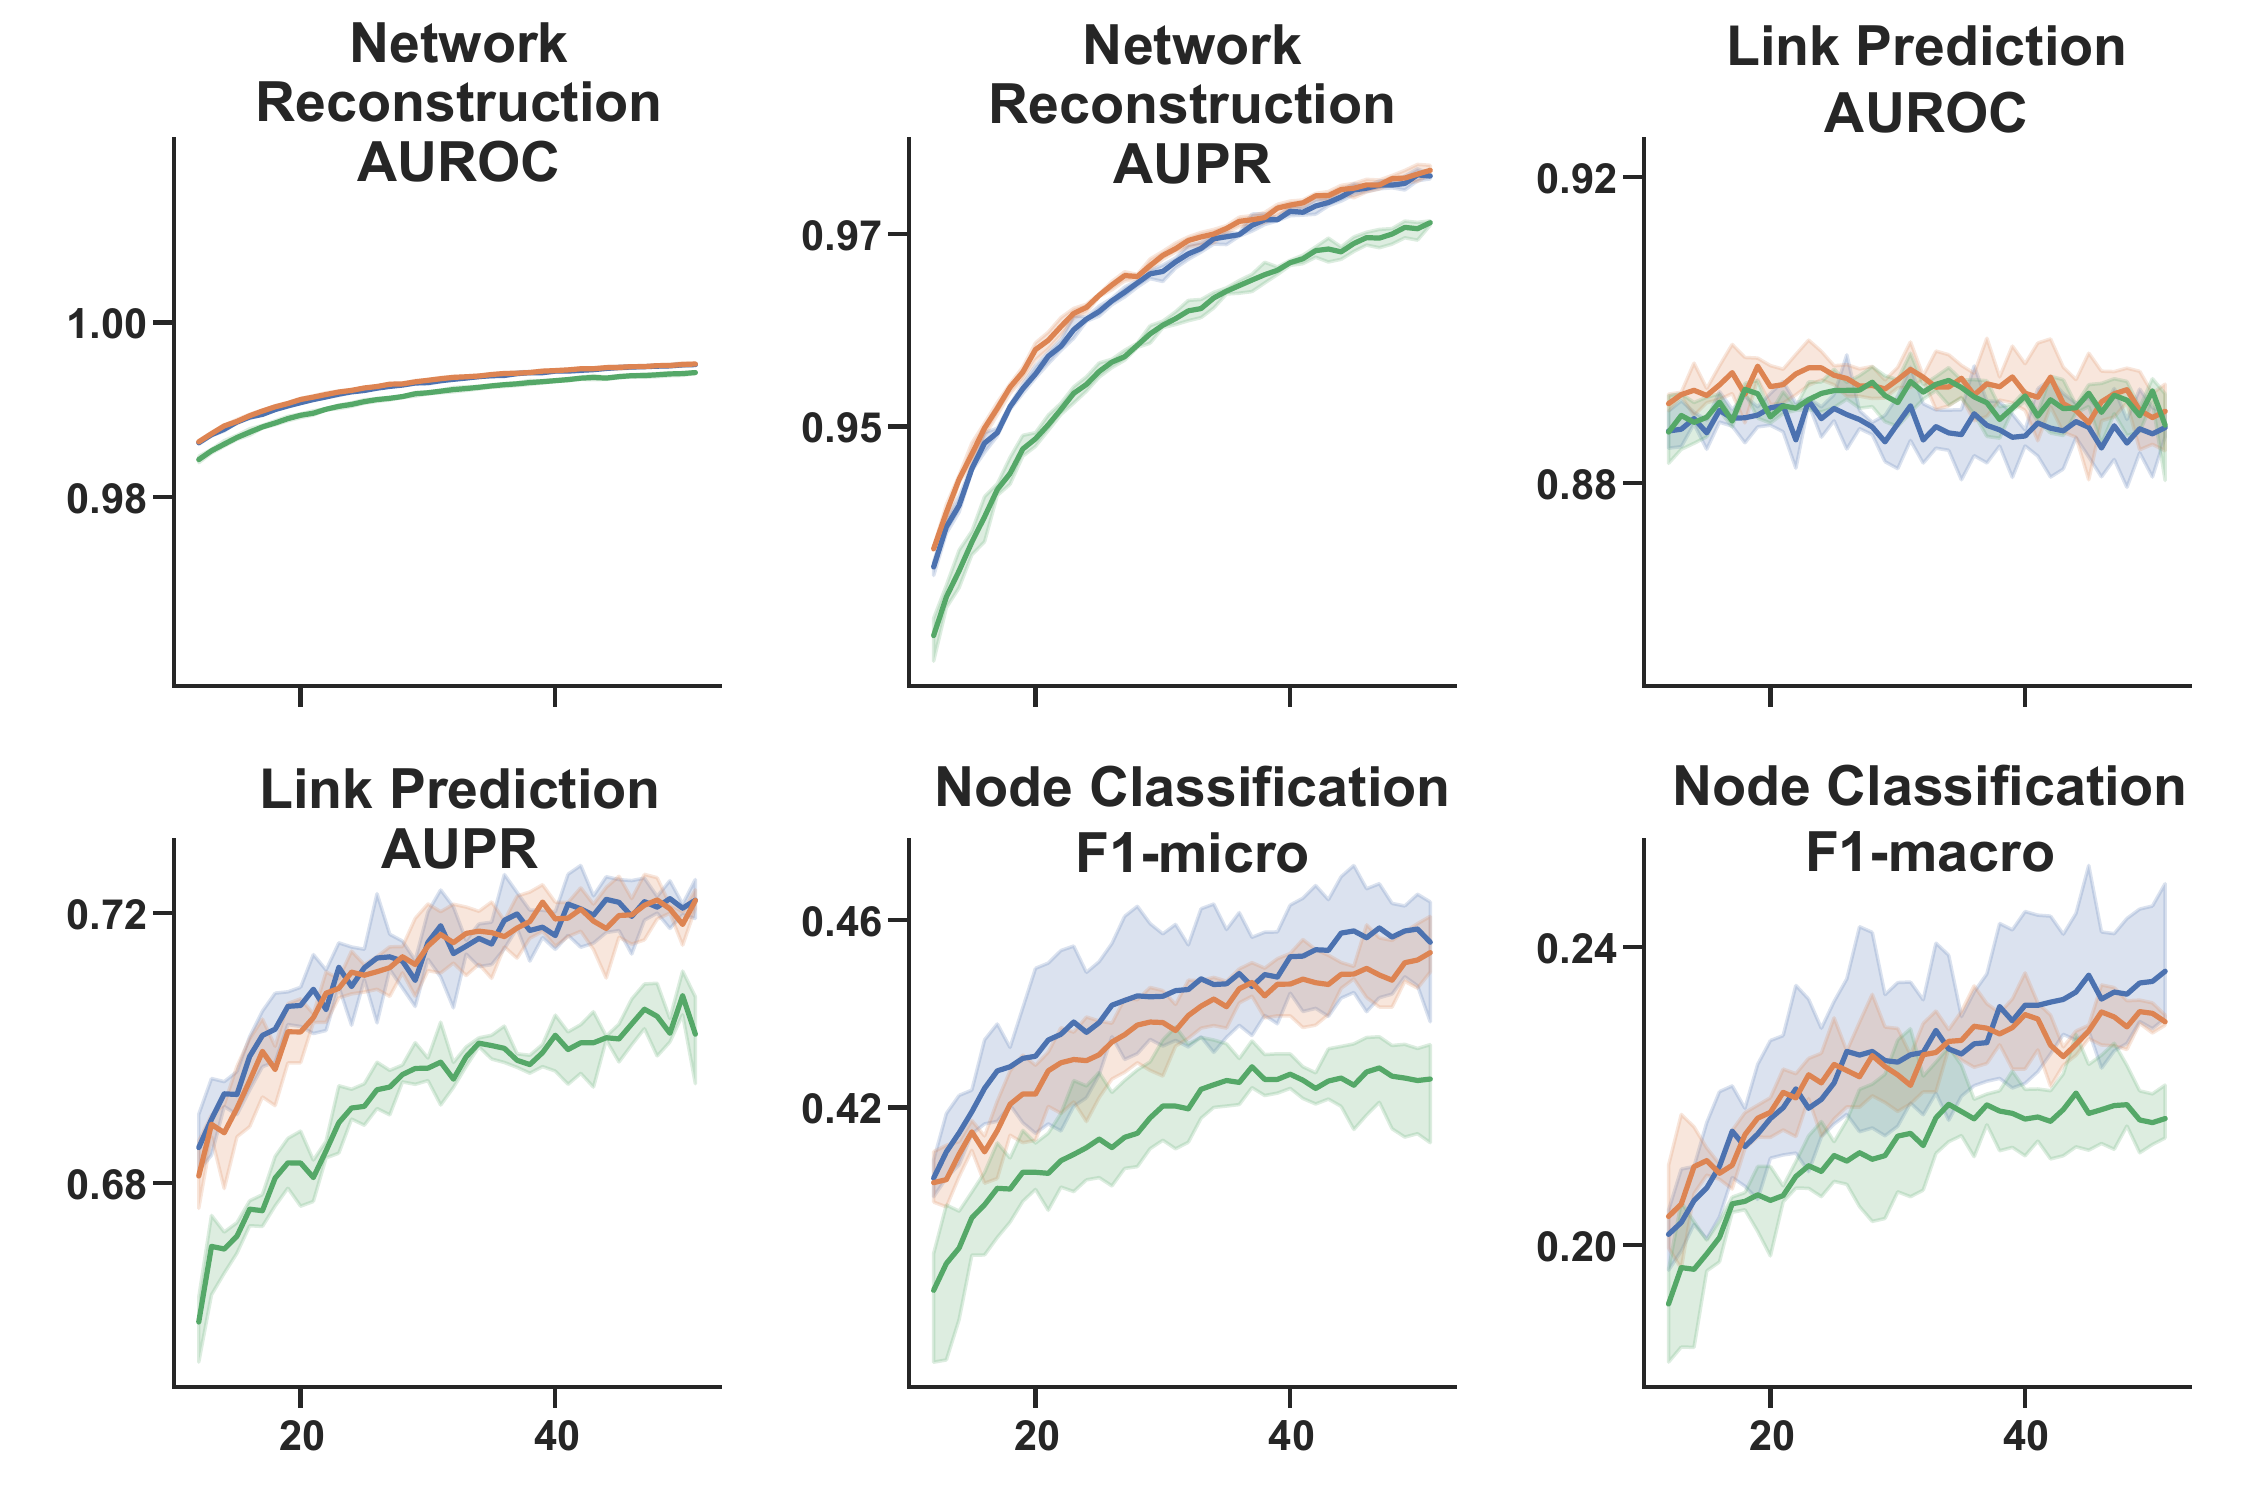}
    \caption{Performance Comparison of Our Model - Encoder and Variant Type I, II(wordnet)}
    \label{fig:perform_wordnet2}
\end{figure}

First, for our model with the random walk. 
Our model is the best in terms of all metrics for the GPS, MovieLens and wordnet dataset.
On the drug dataset, our model achieves higher AUROC and AUPR score on the network reconstruction task than two variants, but slightly lower AUROC score for the link prediction task (less than 0.5\%). 

Then for our model with the encoder, the advantage is not that obvious. 
All 3 methods achieve similar performance in terms of all metrics for the GPS and the drug dataset. 
For the MovieLens and wordnet dataset, our model performs similar to variant type I, higher than variant type II on the network reconstruction and link prediction task. 
But, our model achieves slightly higher accuracy on the node classification task than variant type I.

To sum up, these tests demonstrate that the choice of the structure of our model can achieve higher or at least comparable performance that the 2 potential variants over multiple tasks on multiple datasets.
